# Supplementary material for: Auditing and Enforcing Conditional Fairness via Optimal Transport
Source: arXiv:2410.14029 source file (2024-10-17)
Supplement: Supplementary file 1 [file additional_numerical.tex]

\luhao{Cross Entropy, Reg: f(x), Unfairness: f(x), ACC: 4 measures of accuracy}
\begin{figure}[!htb]
    \centering
    \begin{minipage}{.5\textwidth}
        \centering
        \includegraphics[width=\linewidth]{figure/loan-AUC-diff/conditional_statistical_parity_l1-accuracy.png}
        % \caption{$dt=0.1$}
        % \label{fig:loan:SP}
    \end{minipage}%
    \begin{minipage}{0.5\textwidth}
        \centering
        \includegraphics[width=\linewidth]{figure/loan-AUC-diff/conditional_statistical_parity_l1-AUROC.png}
        % \caption{$dt =$}
        % \label{fig:loan:CSP1}
    \end{minipage}
\end{figure}
\begin{figure}    
    \begin{minipage}{.5\textwidth}
        \centering
        \includegraphics[width=\linewidth]{figure/loan-AUC-diff/conditional_statistical_parity_l1-cross_entropy.png}
        % \caption{$dt=0.1$}
        % \label{fig:loan:CSP2}
    \end{minipage}%
    \begin{minipage}{0.5\textwidth}
        \centering
        \includegraphics[width=\linewidth]{figure/loan-AUC-diff/conditional_statistical_parity_l1-MSE.png}
        % \caption{$dt =$}
        % \label{fig:loan:CSPI}
    \end{minipage}
    \caption{Demonstration of the trade-off between different measures of accuracy and fairness (CSP-$\ell_1$).}
    % \label{fig:loan:CSP}
\end{figure}

\begin{figure}[!htb]
    \centering
    \begin{minipage}{.5\textwidth}
        \centering
        \includegraphics[width=\linewidth]{figure/loan-iter/CSP_Infinity-5.png}
        % \caption{Bi-causal}
        % \label{fig:loan:SP}
    \end{minipage}%
    \begin{minipage}{0.5\textwidth}
        \centering
        \includegraphics[width=\linewidth]{figure/loan-iter/CSP_Infinity-2.png}
        % \label{fig:loan:CSP1}
    \end{minipage}
    \caption{Demonstration of $\mathsf{CSP}_f^{\infty}$ (right) for each iterations as $\lambda$ changes for Bi-causal(left) and Sinkhorn (right), training with gradient descent.}
\end{figure}
\begin{figure}[!htb]
    \begin{minipage}{.5\textwidth}
        \centering
        \includegraphics[width=\linewidth]{figure/loan-iter/CSP_Infinity-3.png}
        % \caption{Bi-causal with batches}
        % \label{fig:loan:CSP2}
    \end{minipage}%
    \begin{minipage}{0.5\textwidth}
        \centering
        \includegraphics[width=\linewidth]{figure/loan-iter/CSP_Infinity-4.png}
        % \caption{Energy distance with batches}
        % \label{fig:loan:CSPI}
    \end{minipage}
    \caption{Demonstration of $\mathsf{CSP}_f^{\infty}$ (right) for each iterations as $\lambda$ changes for Bi-causal(left) and Energy distance (right), training with stochastic gradient descent with batch size $1000$.}
    % \label{fig:loan:CSP}
\end{figure}

\newpage
\luhao{Cross Entropy, Reg: f(x), Unfairness: f(x), ACC: 4 measures of accuracy, $X=\varepsilon_1+\varepsilon_2$ where $\varepsilon_1 \sim Uniform (0,5)$, $\varepsilon_2 \sim \mathcal N (0, 0.1 \exp(A))$}

\begin{figure}[!htb]
    \centering
    \begin{minipage}{.33\textwidth}
        \centering
        \includegraphics[width=\linewidth]{figure/loan-cov/conditional_statistical_parity_l1-accuracy.png}
        % \caption{Bi-causal}
        % \label{fig:loan:SP}
    \end{minipage}%
    \begin{minipage}{0.33\textwidth}
        \centering
        \includegraphics[width=\linewidth]{figure/loan-cov/conditional_statistical_parity_l2-accuracy.png}
        % \label{fig:loan:CSP1}
    \end{minipage}
    \begin{minipage}{0.33\textwidth}
        \centering
        \includegraphics[width=\linewidth]{figure/loan-cov/conditional_statistical_parity_linfty-accuracy.png}
        % \label{fig:loan:CSP1}
    \end{minipage}
    \caption{Demonstration of the trade-off between measures of accuracy rate and fairness.}
\end{figure}

\luhao{Another set of experiments with same setups}
\begin{figure}[!htb]
    \centering
    \begin{minipage}{.4\textwidth}
        \centering
        \includegraphics[width=\linewidth]{figure/loan-cov/1-conditional_statistical_parity_l1-accuracy.png}
    \end{minipage}%
    \begin{minipage}{0.4\textwidth}
        \centering
        \includegraphics[width=\linewidth]{figure/loan-cov/1-conditional_statistical_parity_l2-accuracy.png}
    \end{minipage}
\end{figure}
\begin{figure}[!htb]
\centering
    \begin{minipage}{0.4\textwidth}
        \centering
        \includegraphics[width=\linewidth]{figure/loan-cov/1-conditional_statistical_parity_linfty-accuracy.png}
    \end{minipage}
    \begin{minipage}{0.4\textwidth}
        \centering
        \includegraphics[width=\linewidth]{figure/loan-cov/1-statistical_parity-accuracy.png}
    \end{minipage}
    \caption{Demonstration of the trade-off between measures of accuracy rate and fairness.}
\end{figure}
